# Supplementary material for: Newton: A Language for Describing Physics
Source: arXiv:1811.04626 source file (2018-11-12)
Supplement: Supplementary file 1 [file appendix-b.tex]

\section{Appendix: EBNF Grammar for the Newton}
\label{FormalGrammar}
\lstinputlisting[tabsize=8]{newton.grammar}
